# Supplementary material for: Local composition fluctuations act as precursors for crystal nucleation in polydisperse hard spheres
Source: arXiv:2512.20300 ancillary file (2025-12-23)
Supplement: Supplementary file 1 [file SI_Nucleation_polydisperse_HS.pdf]

# Supplementary Material for "Local composition fluctuations act as precursors for crystal nucleation in polydisperse hard spheres"

Marjolein de Jager,[1] Antoine Castagnède,[2] Frank Smallenburg,[2] and Laura Filion[1]

[1]*Soft Condensed Matter and Biophysics, Debye Institute for Nanomaterials Science, Utrecht University, 3584 CC Utrecht, Netherlands*

[2]*Université Paris-Saclay, CNRS, Laboratoire de Physique des Solides, 91405 Orsay, France*

This Supplementary Material includes the values of the fit parameters for the nucleation rates and the additional analysis on the radial composition of crystal nuclei of polydisperse hard spheres. Additionally, we include plots of the nucleation barriers used to calculate the nucleation rates using umbrella sampling.

## I. NUCLEATION RATE FITS

We fit the nucleation rates in Fig. 1 of the main paper using a fit based on classical nucleation theory (CNT), see Eq. 4 of the main paper. In Tab. S1, we report the specific values of the fit parameters $a$ and $b$ of these fits.

TABLE S1. Fit parameters $a$ and $b$ for the CNT-like fits shown in Fig. 1 of the main paper.

| Polydispersity (%) | $\log(a)$ | $b$ |
|---|---|---|
| 0 | $5.90 \pm 0.17$ | $0.0419 \pm 0.0003$ |
| 1 | $5.46 \pm 0.17$ | $0.0415 \pm 0.0003$ |
| 2 | $6.25 \pm 0.26$ | $0.0440 \pm 0.0005$ |
| 3 | $6.47 \pm 0.36$ | $0.0458 \pm 0.0008$ |
| 4 | $6.36 \pm 0.66$ | $0.0480 \pm 0.0014$ |
| 5 | $7.46 \pm 0.54$ | $0.0540 \pm 0.0012$ |
| 6 | $8.05 \pm 1.78$ | $0.0611 \pm 0.0044$ |

## II. NUCLEATION BARRIERS

We report in the main paper the nucleation rates obtained from umbrella sampling (US) simulations. In Fig. S1, we show the averaged barriers obtained from 10 independent sets of simulations. The standard error amounts to $\sim 1k_BT$ at the top of the barrier.

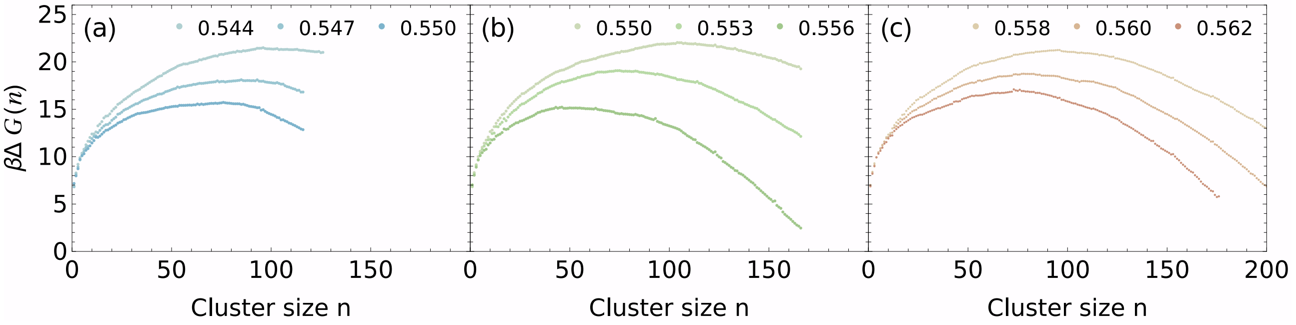


FIG. S1. Nucleation barriers obtained from umbrella sampling simulations of 10000 particles at (a) 4%, (b) 5%, and (c) 6% polydisersity. The different colored points indicate different packing fractions of the system.

## III. RADIAL COMPOSITION

In the main paper (when discussing the results of Fig. 3), we suggest that preference of nuclei for larger particles diminishes once the nucleus enters the growth stage. Here, we provide further evidence of this by examining the

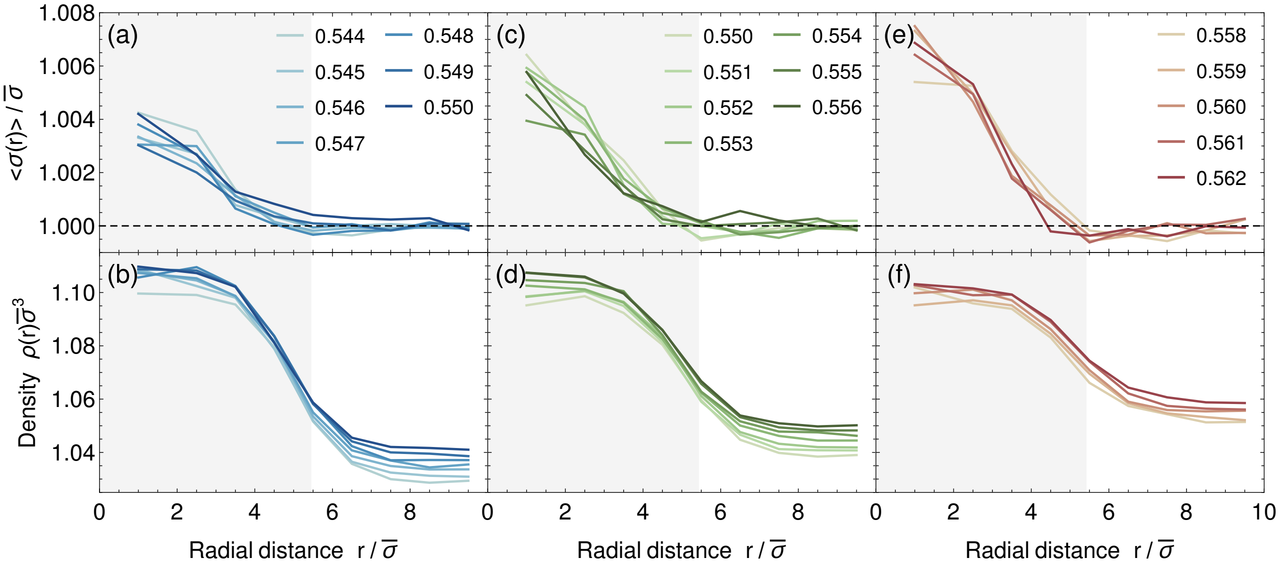


FIG. S2. The average radial trends of (a,c,e) the composition and (b,d,f) the density for (a,b) 4%, (c,d) 5%, and (e,f) 6% polydispersity. These radial trends are taken from the center of mass of the crystal nucleus, and only nuclei containing between 600 and 820 particles are considered. The different colored lines indicate different packing fractions of the system, and the light gray shading indicates the approximate radial size of a sphere of 700 particles.

radial composition of the crystal nuclei. In Fig. S2, we present the average radial profiles of the state points studied for 4%, 5%, and 6% polydispersity. These average profiles are obtained from snapshots of larger nuclei, specifically those containing between 600 and 820 particles. As expected, the average particle size inside the crystal nucleus is larger than in the surrounding fluid. However, we find that preference for larger particles decreases sharply after approximately $2.5\bar{\sigma}$, well before the crystal–fluid interface, as indicated by the density profile. Notably, a sphere with a radius of 2.5 to $2.8\bar{\sigma}$ contains around 70-100 particles, which roughly corresponds to the size of the critical nucleus for the state points studied. Thus, we can indeed conclude that, during the growth stage, the nucleus essentially absorbs any neighboring fluid particle, regardless of size.
